# Supplementary material for: Starting from the amorphous ground state: linking landscape thermodynamics to slow dynamics and crossover
Source: arXiv:2307.10143 ancillary file (2026-05-22)
Supplement: Supplementary file 1 [file FSC_SI.pdf]

# Supplementary Information: Depleting states dictate the ideal glass and physics of glass transition

Anshul D. S. Parmar<sup>1,2,\*</sup> and Andreas Heuer<sup>1,†</sup>

<sup>1</sup>*Institute of Physical Chemistry, Westfälische Wilhelms-Universität Münster,  
Corrensstraße 28/30, 48149 Münster, Germany*

<sup>2</sup>*Helmholtz-Institute Münster (IEK-12) Forschungszentrum Jülich GmbH,  
Corrensstraße 46, 48149 Münster, Germany*

---

\* aparmar@uni-muenster.de

† andheuer@uni-muenster.de

Here we provide additional information about the following topics: (I) Discrete-polydisperse system, (II) Sampling in perfect equilibrium, (III) Structural information via pair correlation function, (IV) Inherent structure energies for various system sizes, (V) Participating particles in the relaxation process, (VI) Characterization of the dynamics, (VII) The temperature associated with the identification of the bottom of the PEL, (VIII) Low energy spectrum near the cutoff, (IX) The configurational entropy (X) Finite-size effects (XI) Observations in experimental systems for the FSC.

## I. DISCRETE-POLYDISPERSE SYSTEM

For a range of the system sizes examined in the investigation, we study the discrete-polydisperse system with  $M = 10$  types of particles following the  $P(\sigma) \propto \sigma^{-3}$  distribution(Fig. 1(a)). We observe that the compositions  $M = 10$  do not largely affect the efficiency of the swap Monte-Carlo at low temperatures(Fig. 1(b)) and provide well-relaxed samples for the relevant temperatures range for studying the potential energy landscape.

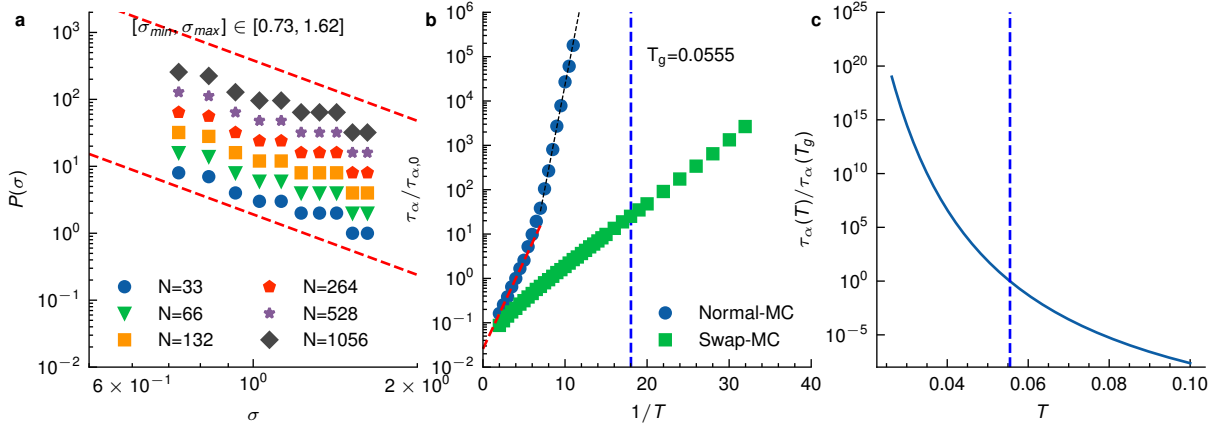

FIG. 1. **Discrete choices for the particle sizes.** **a** The particle size distribution for the continuous(fit lines) and the utilized discrete choice of particle type (symbols). **b** The speedup summary for the 1056 particles for the  $M=10$  and **(c)** temperature vs. extrapolated the MC-relaxation time, from the Arrhenius fit the normal MC-time, suggesting effective swap dynamics till the low-temperature regime.

To understand the relaxation, we study the intermediate scattering function to quantify

the structural relaxation for swap dynamics.

$$F_s(\mathbf{k}, t) = \frac{1}{N} \left\langle \sum_{i=1, N} \exp[i\mathbf{k} \cdot (\bar{\mathbf{r}}_i(t) - \bar{\mathbf{r}}_i(0))] \right\rangle \quad (1)$$

at the momenta  $|\mathbf{k}| (= 2\pi)$  corresponding to the first peak of the static scattering factor. To negate the long wavelength Mermin-Wagner fluctuations in 2D systems, we utilize the relative positions  $\bar{\mathbf{r}}$ . The structural relaxation time  $\tau_\alpha$  corresponds to the decay of  $1/e$  of the intermediate scattering function. The angular brackets represent the average over independent measurements and possible components of momenta. The glass transition temperature  $T_g = 0.0555$  is marked by 12-decade glassy structural relaxation dynamics, extrapolating with the Arrhenius relation for the normal-MC. Fig. 1(c) shows the parametric plot for the temperature and the structural relaxation time from the Arrhenius fit, highlighting  $10^{19}\tau_\alpha(T_g)$  of the relaxation time.

## II. SAMPLING IN PERFECT EQUILIBRIUM

To test the equilibration for the system via swap Monte-Carlo simulations, we

- i* inspect aging,
- ii* compare the relaxation via particle motion and size auto-correlation in swap dynamics, and
- iii* an independent quantification of the relaxation via PEL.

In Fig 2(a), we report the  $F_s(\mathbf{k}, t)$  for the equilibrated samples across the  $T_g$  including temperature at the cutoff in the PEL is observed, and corresponding waiting (swap MC) time ranging from  $t_W \in [2^0, 2^{18}]$ . The samples do not exhibit any aging throughout the study.

We observe the correlation between positional dynamics and diameter for quantifying structural relaxation. The positional dynamics is the system's evolution in real space due to the swap moves, whereas the autocorrelation function provides an entirely independent test for relaxation from diameter fluctuations [1], defined as

$$C_\sigma(t) = \langle c_\sigma(t) \rangle = \left\langle \frac{\sum_i \delta\sigma_i(t) \delta\sigma_i(0)}{\sum_i \delta\sigma_i^2(0)} \right\rangle, \quad (2)$$

where  $\delta\sigma_i(t) = \sigma_i(t) - \sigma_i(0)$  and the function is normalized with the correlation at time zero. Fig. 2 (b) shows structural relaxation from the position and the diameter, and the relaxation time for  $C_\sigma(t)$  is scaled to the  $F_s(k, t)$  for  $T=0.1053 (\approx T_{MCT})$ . The systematic decay in  $C_\sigma(t)$  represents that diameters become entirely uncorrelated from their initial values, even for a smaller system with 10 particle types. The excellent agreement between the structural relaxation from the position and the diameter, suggests samples are adequately relaxed.

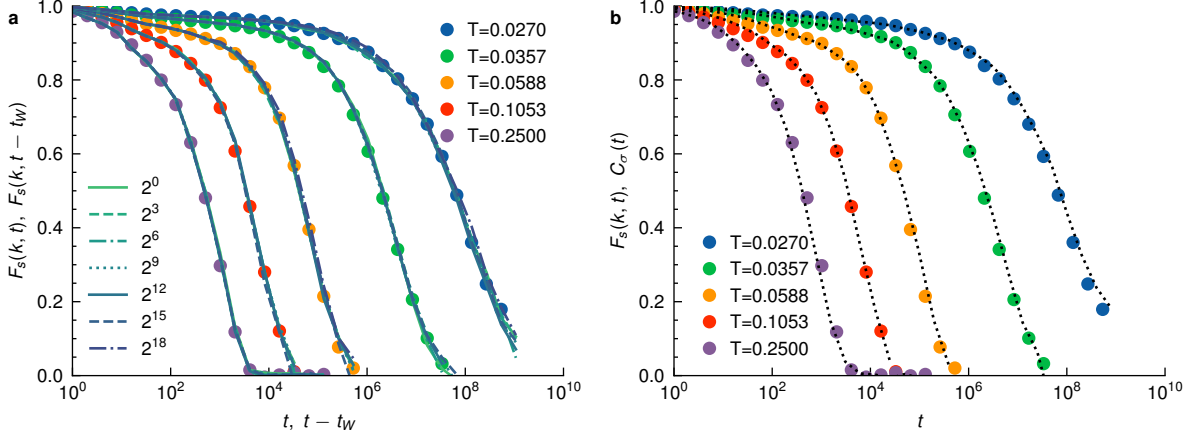

FIG. 2. **Aging and relaxation** **a** The samples do not show noticeable waiting time dependence in the intermediate scattering factor, demonstrating well-relaxed samples. **b** Autocorrelation of particle diameters and intermediate scattering factor measured during the swap dynamics for a wide temperature range, for  $N=66$ .

We perform a stringent test to quantify the sampling from the swap Monte-Carlo simulation representing the PEL from the equilibrium. The weighted distribution for a given temperature can be expressed as

$$P_W(T, E_{IS}) = P(T, E_{IS}) \exp(\beta E_{IS}). \quad (3)$$

The energy-wise ratio of the weighted distribution, for adjacent temperature, defined as

$$\chi(E_{IS}) = P_W(T_i, E_{IS}) / P_W(T_j, E_{IS}). \quad (4)$$

The ratio  $\chi(E_{IS})$  studied from the high temperature  $T = 0.2 (< T_{onset})$  down to the lowest chosen temperature for each system. Fig. 3 shows a constant ratio( $\chi$ ) across each energy interval, ensuring the equilibrium sample towards very low temperatures.

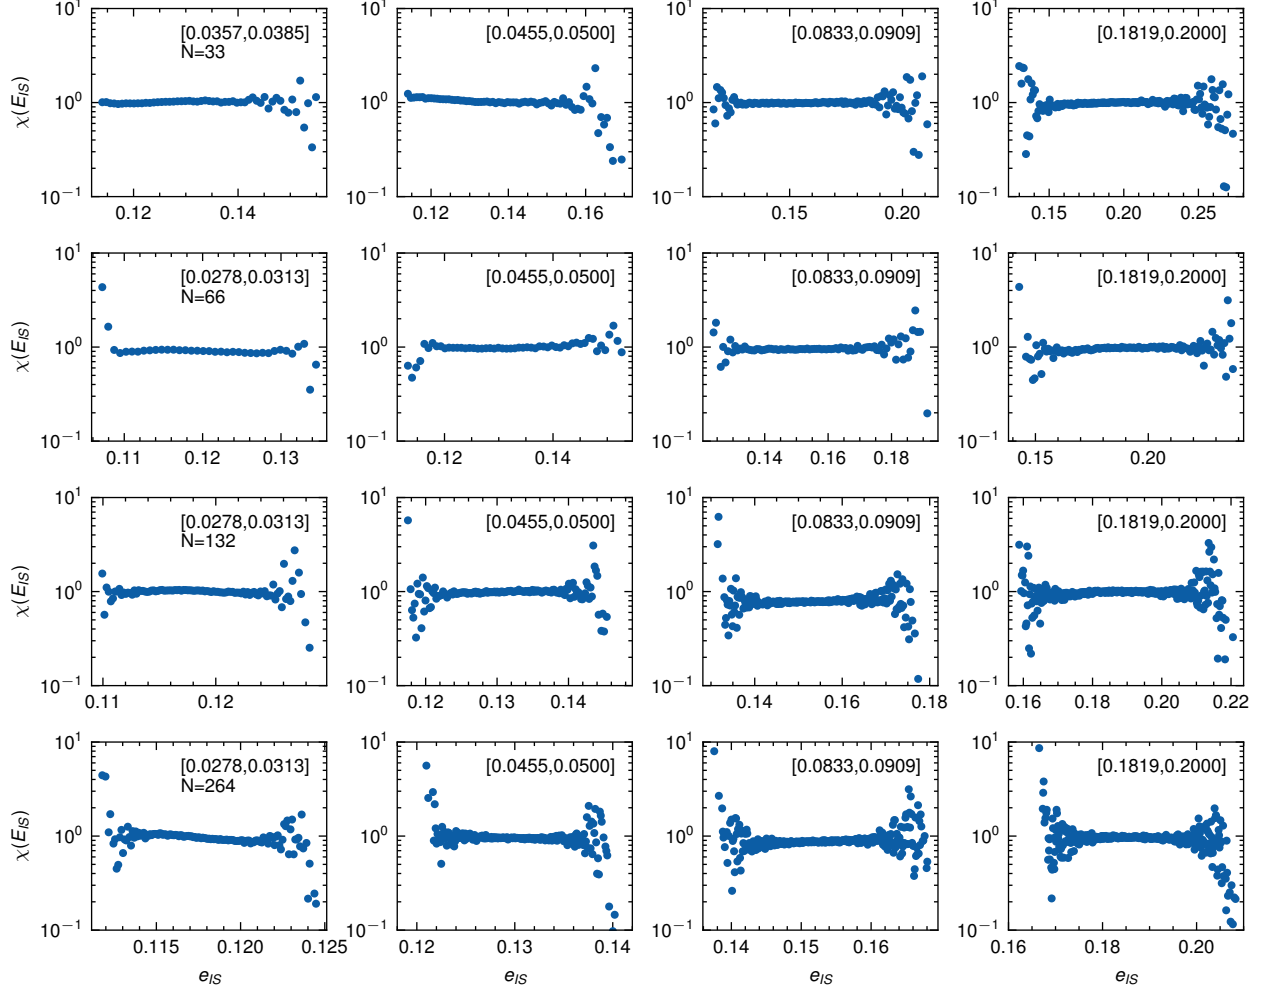

FIG. 3. **The ratio for the weighted distribution.** The constant ratio for weighted distribution across the range of energy indicates good sampling for the equilibrium study for high temperature to the multi-billion year's relaxation below the  $T_g$ .

### III. STRUCTURAL INFORMATION VIA PAIR CORRELATION FUNCTION

Using the pair correlation function( $g(r)$ ), we can quantify how the particle of interest is surrounded by others. We study a range of system sizes  $N \in [33, 1056]$  for  $M = 10$  at  $T=0.050$ , corresponding to a deeply supercooled state below  $T_g$ . Fig. 4 suggests that even the smallest system, consisting of 33 particles, contains at least two coordination shells. The particles  $i$  and  $j$  are neighbors from the first coordination shell if the distance  $r_{ij} \leq 1.33\sigma_{ij}$  is used to calculate the relative displacements of cages.

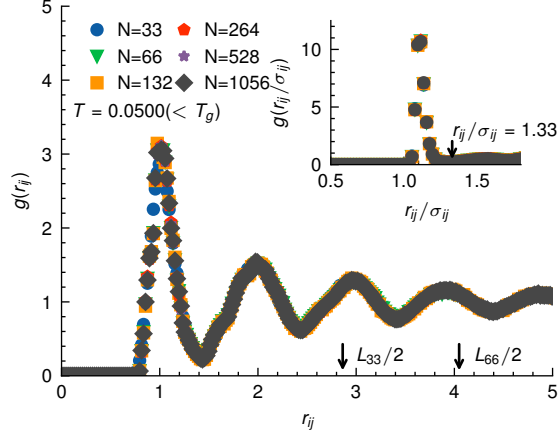

FIG. 4. **Structure.** The pair correlation function of the inherent structures for various system sizes at the  $T=0.0500$ . The vertical arrows represent half of the box length, suggesting that even for  $N=33$  particles, the box contains at least two coordination shells. The insets show the radial distribution function for the scaled distances ( $r_{ij}/\sigma_{ij}$ ). The vertical arrow represents the cutoff choice for the neighbors.

#### IV. INHERENT STRUCTURE ENERGIES FOR VARIOUS SYSTEM SIZES

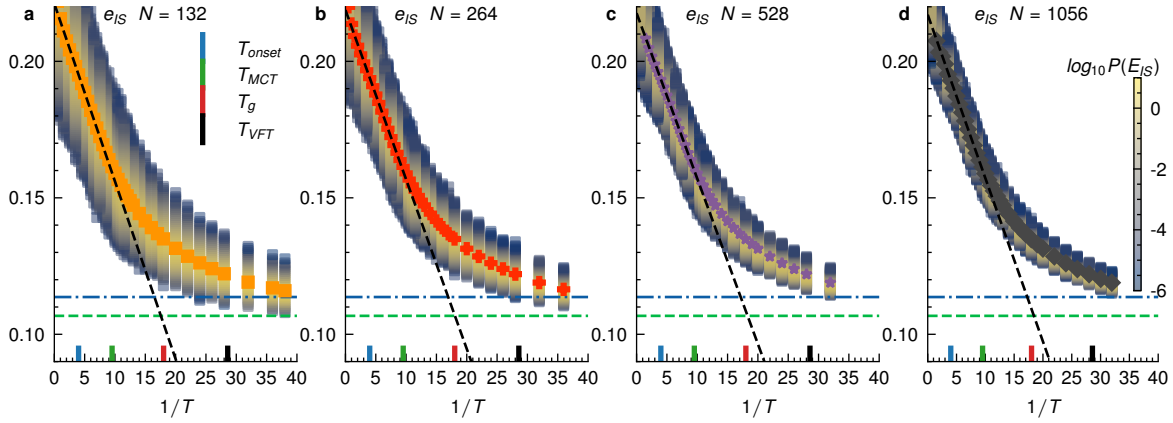

FIG. 5. **PEL vs. system size.** The mean  $e_{IS}$  for various system sizes. Notably, while a high-temperature regime exhibits Gaussian behavior, we observe a low-temperature asymptotic behavior in the energy that remains consistent across all system sizes. The lowest energy levels for system sizes  $N=33$  and  $N=66$  are depicted by the dot-dashed and dashed lines, respectively.

In our study, we have systematically observed the non-Gaussian nature of the Potential Energy Landscape (PEL) across various system sizes (see Fig. 5a-d). As expected, the

statistical fluctuations for the energy per particle become smaller for larger  $N$ .

## V. PARTICIPATING PARTICLE IN RELAXATION PROCESS

To explore the influence of the system sizes on the dynamics, we study the localization of particle rearrangements resulting from IS-IS transitions. For this purpose, we measure the number of involved particles in the IS-IS transition by the participation ratio (PR), defined as

$$PR = \frac{[\sum_{i=1,N} d\bar{\mathbf{r}}_{i,IS}^2]^2}{\sum_{i=1,N} (d\bar{\mathbf{r}}_{i,IS})^4}, \quad (5)$$

where  $\bar{\mathbf{r}}$  represents the case relative displacement in the IS-IS transition. In the IS-IS event, the PR would yield the total mobile particles involved in the transition.

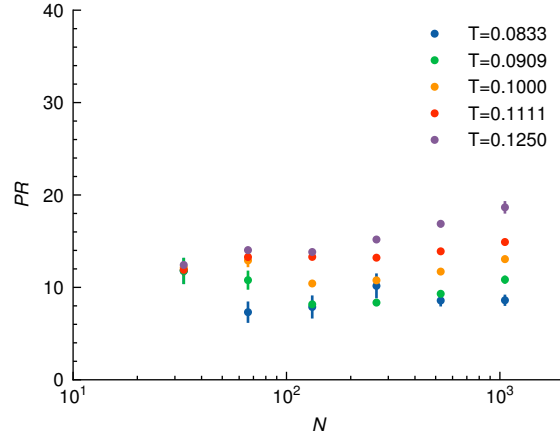

FIG. 6. **Participation ratio across the system sizes.** Mean participation ratio (PR) for a range of the system sizes across the  $T_{MCT} = 0.105$  characterizing the number of particles participating in the rearrangements in the transitions between successive inherent structures. The vertical lines correspond to the standard error.

Fig. 6 shows the PR, averaged over 100 IS-IS transitions for a range of system sizes and temperatures across  $T_{MCT}$ . As temperature decreases, the IS dynamics become more localized, resulting in fewer mobile particles. Again, for  $N \geq N_c = 66$ , we hardly see any finite-size effects.

## VI. CHARACTERIZATION OF THE DYNAMICS

The system's dynamics are characterized by the temperature of diffusion( $D$ ) and structural relaxation( $\tau_\alpha$ ) time for various systems. At the high temperature, the system exhibits the well-observed Arrhenius relation, defined as

$$X(T) = X_\infty \exp(-\beta A_H), \quad (6)$$

where the symbol  $X$  defines the inverse diffusion/ structural relaxation time,  $X_\infty$  depicts infinite temperature dynamics, and  $A_H$  corresponds to the high-T activation energy. The deviation from the high-temperature Arrhenius behavior marks the onset temperature( $T_{onset} = 0.25$ ), beginning with the supercooled dynamics.

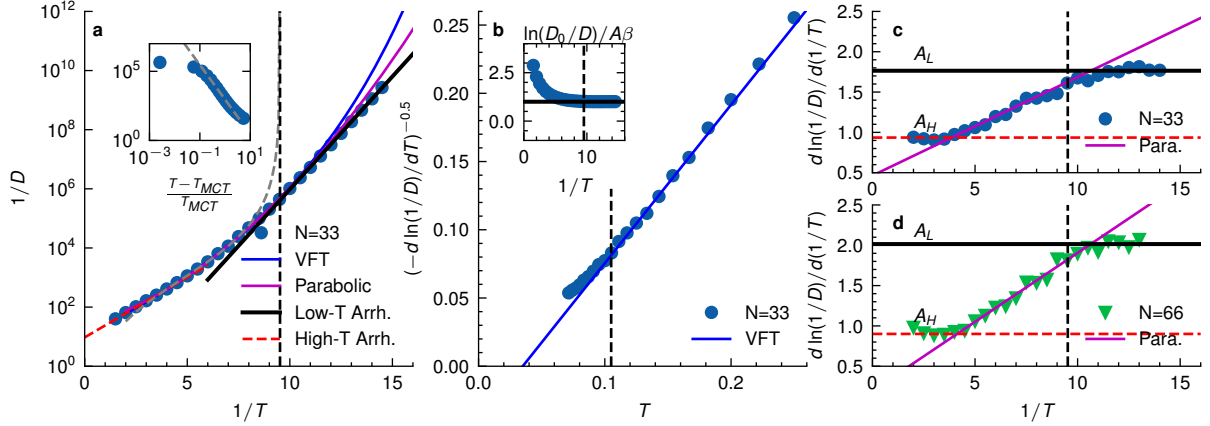

FIG. 7. **Summary of the dynamics for N=33 and 66.** **a** The inverse diffusion vs. inverse temperature, covering roughly 7 decades of glassy relaxation. The diffusion coefficient is further used to estimate the MCT temperature and describe the VFT, and parabolic description of the dynamics. The MCT fit is performed for  $T \in [0.1333, 0.25]$  and VFT and parabolic fitting for  $T \in [0.1111, 0.25]$ . The vertical line marks the  $T_{MCT} = 0.105$ , and the inset represents the linearized form of the MCT relation. The linearized form of the **(b)** VFT and **(c, d)** parabolic function highlights the clear deviation at the low temperature. (inset, **b**) A clear Arrhenius relation below the temperature 0.1, marking the FSC. **c & d** Horizontal lines mark high and low-temperature activation energies. **d** Highlighting the consistency between N=66 and N=33, with slightly higher activation energy at low temperatures.

Next, we define the mode-coupling temperature for the system, the finite temper power-

law divergence predicted as

$$X(T) \propto |T - T_c|^{-\gamma}, \quad (7)$$

where  $T_c$  and  $\gamma$  represent the mode-coupling temperature and exponent, respectively. Experiments and simulations show deviations from the mode-coupling theory(MCT), generally referred to as MCT crossover.

In addition to the MCT crossover, the dynamics can be described by the Vogel-Fulcher-Tammann (VFT) equation, which accounts for a finite temperature divergence(VFT) [2], defined as

$$X(T) = X_\infty \exp \left[ \frac{1}{K_{VFT}(T/T_{VFT} - 1)} \right], \quad (8)$$

where  $X_\infty$ ,  $K_{VFT}$ , and  $T_{VFT}$  represent infinity-temperature dynamics, kinetic fragility, and finite temperature divergence, respectively.

Another description of the dynamics can be defined as the parabolic fit, considered the most straightforward correction to the Arrhenius behavior that includes dynamic fragility [3]. The zero temperature divergence for the parabolic fits can be defined as

$$X(T) = X_o \exp \left[ J \left( \frac{1}{T} - \frac{1}{T_o} \right)^2 \right], \quad (9)$$

where  $T_o$  and  $X_o$  represent the onset temperature and dynamics, respectively. The fit parameter  $J$  represents the temperature-dependent kinetic fragility. It is noteworthy that both the VFT and parabolic descriptions predict a systematic increase in the activation energy as the system is cooled.

In Fig. 7(a), we discuss the aforementioned fits to provide a comparative description of dynamics. The MCT crossover temperature,  $T_{MCT}$ , is marked with the MCT fit (see eq. VI) for the first two decades of diffusion below  $T_{onset}$ . Fig. 7(inset) shows the linearized form of MCT to represent the crossover and fit quality. We next discuss the VFT and parabolic fits for the diffusion from 3 decades of supercooled liquid below the  $T_{onset}$ . The fig. 7(b-d) compares the linearised fit-free form with the raw data. The data, spanning 7-decades of diffusion, show a clear deviation from the VFT and parabolic dependence of the dynamics. The low-temperature Arrhenius behavior provides strong evidence of fragile-to-strong crossover at the low temperature (see linearized form in the inset of fig. 7).

Our findings are consistent for the largest system ( $N = 1056$ ) as well. Fig. 8(a) reports the diffusion and the structural relaxation for a large range of temperatures. The extremely

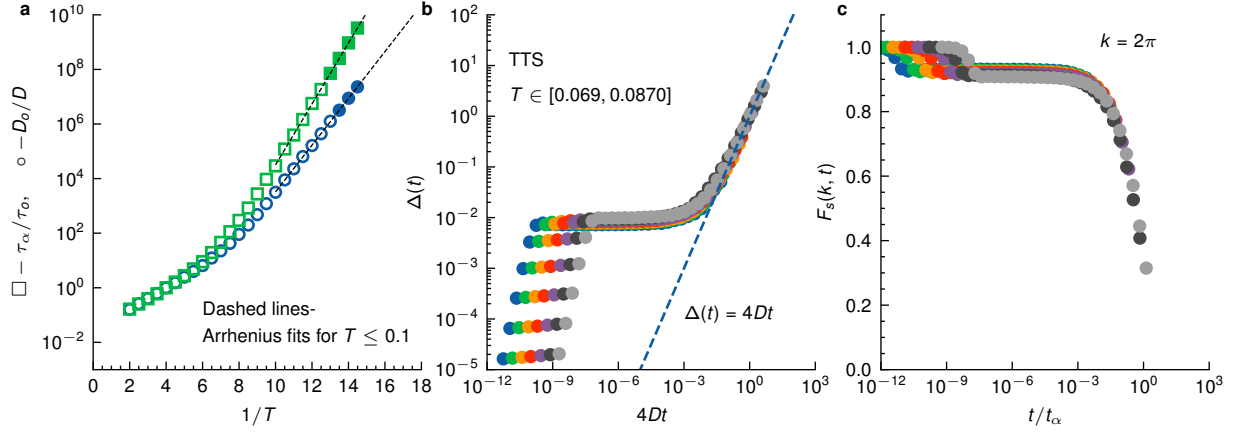

FIG. 8. **Summary of the dynamics for  $N = 1056$ .** **a** The inverse diffusion and relaxation time (scaled to onset temperature,  $T_{onset}$ ) vs. inverse temperature, covering roughly 7 and 10 decades of equilibrium relaxation, respectively. Filled symbols correspond to the extrapolated dynamics, using the time-temperature scaling (**b** & **c**).

long runs for low temperatures allow us to test the estimates for the Arrhenius dependence of the dynamics and the time-temperature scaling [4] (as shown in fig. 8(b & c)). The 4-5 decades of low-temperature Arrhenius behavior suggest that our findings are consistent across the system sizes and dynamical measurements.

Note the same onset temperature behavior for diffusion and structural relaxation. Due to the dynamical heterogeneities at the low temperature, the diffusion coefficient and the structural relaxation time decouple. i.e.,  $D \propto \tau_\alpha^{-\xi}$ , where  $\xi$  is the Stokes-Einstein breakdown (SEB) exponent [5]. For the current system, the SEB exponent is 0.77, which results in slightly different activation energies ( $A_D = \xi A_{\tau_\alpha}$ ).

## VII. THE TEMPERATURE ASSOCIATED WITH THE IDENTIFICATION OF THE BOTTOM OF THE PEL

Identification of a low-energy cutoff is defined by accessing the same lowest energy at equilibrium runs at different temperatures.  $T_{cut}$  denotes the highest temperature where the low-energy cutoff is found. In order to define  $T_{cut}$  without the necessity to take into account random effects, we define it according to the criterion  $P(E_{lowest, IS}, T_{cut}) = p_{cut}$  where  $p_{cut}$  is a fixed value which we choose to be  $10^{-6}$ . This choice is based on the observation that for both

$N = 33$  and  $N = 66$  at  $T_{cut}$ , their empirical probability (i.e., number of occurrences relative to the total number of identified IS) was close to  $10^{-6}$ . Indeed, the resulting temperatures  $T_{cut}$ , see Fig. 9, obtained from this statistical approach, are close to what we found from our simulations (see main text). This shows the consistency of the procedure.

In order to predict  $T_{cut}$  for larger  $N$ , we assume strict validity of the factorization hypothesis, starting when generating the PEL of  $N = 132$  from the PEL of  $N = 66$ . The resulting values of  $T_{cut}$  are shown in Fig. 9. As expected, identification of the bottom of the PEL requires much lower temperatures for larger system sizes. Thus, the difference of  $T_{cut}$  for  $N = 33$  and  $N = 66$  is not only due to the presence of a lower minimum for  $N = 66$  but also due to trivial statistical reasons. Under the idealized assumption that the factorization hypothesis works until the lowest energies, one might thus expect that for  $T \approx T_{cut}$  and similar numerical efforts (in terms of the number of successive IS) the probability is of order one to identify the lowest-energy state. This data also suggest that for a macroscopic system, the lowest energy state can only be accessed in the limit of zero  $T_{cut}$ . However, we would like to stress that this is a purely statistical effect because the relevant system size is the smallest system size where macroscopic behavior is quantitatively observed, i.e., here for  $N = N_c = 66$ .

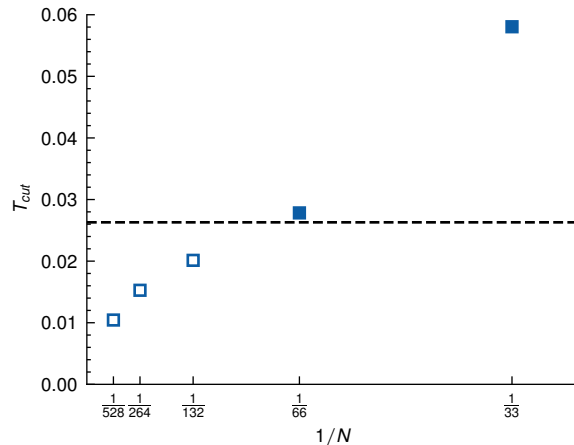

FIG. 9. **The energy-cutoff and system size.** The  $T_{cut}$  vs.  $1/N$  for a large range of system sizes. The horizontal line represents the lowest temperature explored in equilibrium with the swap Monte-Carlo simulation. To estimate  $T_{cut}$  for  $N \geq 132$ (open symbols), the complete IS density has been estimated via the factorization hypothesis.

### VIII. LOW ENERGY SPECTRUM NEAR THE CUTOFF

In fig. 10, we report the lower energy spectrum for the  $N=33$  and  $N=66$ . To illustrate the same energy scale, we shift the energy  $E_{lowest}/N = 0.113652322808157$  and  $E_{lowest}/N = 0.106756393732118$  for  $N=33$  and  $66$ , respectively. For numerical accuracy, two energy levels( $i,j$ ) are considered to be the same, if the difference between  $i$  and  $j$ :  $(|E_{i,IS} - E_{j,IS}|)/N \leq 10^{-14}$ . The well-defined energy difference allows the marking of various low-energy levels and further progresses in a continuous spectrum for higher energy.

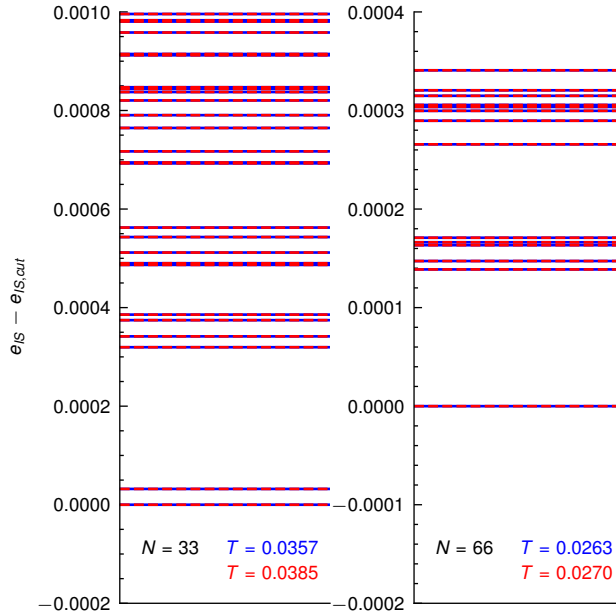

FIG. 10. **PEL near cutoff.** The per-particle energy of the inherent structure highlights the low energy spectrum near the cutoff. The energies are shifted with the bottom to show the same energy range. For  $N=33$  and  $N=66$ , within the relevant Boltzmann weight, the 28 and 16 energy levels are the same across the lowest two temperatures, respectively.

Fig. 10 shows the energy level ( $E_{i,IS}$ ) at the two lowest analyzed temperatures for  $N=33$  ( $T=0.0357$  and  $T=0.0385$ ) and  $N=66$  ( $T=0.0263$  and  $T=0.0270$ ). We display the IS energies with respect to the cutoff energy  $E_{lowest,IS}$  and use the additional criterion  $(E_{i,IS} - E_{lowest,IS}) \leq T$ . In this way, we identify all energies with a relevant Boltzmann weight which are 28 for  $N=33$  and 16 for  $N=66$ . Importantly, all states are found at both temperatures. Thus, our numerically obtained IS statistics are indeed good enough to characterize the bottom of the PEL fully.

## IX. THE CONFIGURATIONAL ENTROPY

### A. Disentangling the total entropy

The total entropy can be written in the canonical ensemble as

$$S(T) = - \int dx P(x, T) \ln[P(x, T)u], \quad (10)$$

where  $u$  corresponds to some phase space factor and the integral is over the complete (2N-2)-dimensional phase space. Formally, this can be written as a sum over all inherent structures, i.e.

$$S = - \sum_i \int_{\Omega_i} dx P(x, i, T) \ln[P(x, i, T)u]. \quad (11)$$

Next, we introduce the conditional probability  $q_i(x)$  that within IS  $i$  the system is at position  $x$ . Furthermore,  $P(E_{i,IS}, T)$  denotes the probability that the system is in IS  $i$  at temperature  $T$ . Then the entropy can be rewritten as

$$S = - \sum_i P(E_{i,IS}, T) \int_{\Omega_i} dx q_i(x) \ln[P(E_{i,IS}, T)q_i(x)u]. \quad (12)$$

Which further can be disentangled as

$$S = - \sum_i P(E_{i,IS}, T) \ln P(E_{i,IS}, T) - \sum_i P(E_{i,IS}, T) \int_{\Omega_i} dx q_i(x) \ln[q_i(x) u]. \quad (13)$$

These two terms have a specific interpretation. The first term is denoted as the configurational entropy

$$S_c(T) = \sum_i P(E_{i,IS}, T) \ln P(E_{i,IS}, T). \quad (14)$$

The second term can be interpreted as the vibrational entropy  $S_{vib}(T)$ , reflecting the volume and shape of the individual basins.

### B. Harmonic approximation

Both for  $S_c(T)$  and  $S_{vib}(T)$ , it is important to characterize the properties of the basins of each IS. A good starting point is the partition sum  $z_i(T) = \int_{\Omega_i} \int dx u \exp(-\beta(E(x) - E_i))$ .

For low temperatures, one may assume that the physical properties are mainly governed by the region around the minimum and thus can be described in the harmonic approximation. This can be explicitly expressed as (setting  $u = 1$ )

$$\begin{aligned} z_{i,harm}(T) &= \int \Pi_\nu dx_\mu \exp \left( -\frac{\beta}{2} \sum_\mu \lambda_{i,\mu} x_\mu^2 \right) \\ &= \Pi_\nu \left( \frac{2\pi}{\beta \lambda_{i,\nu}} \right)^{1/2} = T^{(Nd-d)/2} Y_i, \end{aligned} \quad (15)$$

where

$$Y_i = \Pi_\nu \left( \frac{2\pi}{\lambda_{i,\nu}} \right)^{1/2} = 2\pi^{(Nd-d)/2} \exp \left( -\frac{1}{2} \sum_\nu \ln \lambda_{i,\nu} \right) \quad (16)$$

is proportional to the effective volume of the basins in harmonic approximation. By  $\lambda_\nu$  we denote the eigenvalues of the Hessian in  $d$  dimension,  $\nu = 1, \dots, (Nd - d)$ .

### C. Determination of the configurational entropy

Generally, the probability contains one term  $Y_i$ , reflecting the effective volume of a basin, i.e.

$$P(E_{i,IS}, T) = \frac{Y_i \exp(-\beta E_{i,IS})}{\mathcal{Z}} \quad (17)$$

with the partition sum (for normalization purposes)  $\mathcal{Z} = \sum_i Y_i \exp(-\beta E_{i,IS})$  with  $\beta \equiv 1/k_B T$ , which Boltzmann's constant  $k_B$  is kept as unity. Furthermore, the IS-density  $G(E_{IS})$  is in the main text defined as  $G(E_{IS}) = \sum_i Y_i \delta(E_{IS} - E_{i,IS})$ . The value of  $Y_i$ , determined in harmonic approximation, is given above. Possible anharmonic corrections are discussed in SI (X).

Inserting Eq. 17 into Eq. 14, the configurational entropy can be expressed as

$$S_c(T) = -\langle \ln Y_i \rangle + \beta \langle E_{i,IS} \rangle + \ln \mathcal{Z}, \quad (18)$$

where  $\langle \ln Y_i \rangle = \sum_i P(E_{i,IS}, T) \ln Y_i$ , the contribution of the basin's volume and  $\langle E_{i,IS} \rangle = \sum_i E_{i,IS} P(E_{i,IS}, T)$  is the mean potential energy of the thermodynamically relevant set of IS. Please note that this is invariant towards scaling of the  $Y_i$ , i.e., the transformation  $Y_i \rightarrow \lambda Y_i$ .

Whereas the numerical determination of the expectation values is straightforward, some care must be taken when calculating the partition sum. To reach the low-temperature

limit, the discrete nature of the IS energies has to be taken into account (for  $N = 33$  and  $N = 66$ ). In contrast, for higher energies, a systematic enumeration of all states is no longer possible, so one has to resort to a continuum description. The transition between both levels of description takes place at the energy  $E_{cut}$ . We introduce the energies  $E_{1,bin} = E_{cut} + (1/2)\Delta E$ ,  $E_{2,bin} = E_{cut} + (3/2)\Delta E, \dots$  and define  $G_{j,bin} = \sum_{i \text{ with } E_{i,IS} \in [E_{j,bin} \pm \Delta E/2]} Y_i$  as the contribution of all states between  $E_{j,bin} - \Delta E/2$  and  $E_{j,bin} + \Delta E/2$ . Here we choose  $\Delta E = 0.02$ . Apart from a constant, all  $G_{j,bin}$  can be obtained from the reweighting scheme, described in SI II. This can be done for all  $N$ , although for  $N > 66$ , only the continuous part of  $G(E_{IS})$  is accessible. When choosing, e.g., for  $N = 33$ , a value  $E_{cut} = 3.76$ , for the first energy bin between 3.76 and 3.78, the absolute number of states is accessible due to the systematic identification of all IS in this energy interval (see SI VIII). This fixes the absolute value of  $G_{1,bin}$  and successively for all  $G_{j,bin}$ . Then we can express the volume-weighted density of states as

$$G(E_{IS}) = \sum_{i, E_{i,IS} \leq E_{cut}} Y_i \delta(E_{IS} - E_{i,IS}) + \sum_j G_{j,bin} \delta(E_{IS} - E_{j,bin}). \quad (19)$$

Finally, the partition sum is given as

$$\mathcal{Z} = \int dE G(E_{IS}) \exp(-\beta E_{IS}). \quad (20)$$

An approximation enters via the discrete nature of  $G(E_{IS})$  in the continuous regime. However, if the energy difference between the lowest IS energy and  $E_{cut}$  is significantly larger than  $\Delta E$ , this approximation should be extremely good. This is explicitly shown in fig 11 both for  $N = 33$  and  $N = 66$ . Specifically, in fig 11(a&d), we show the respective volume-weighted density of states. The arbitrary scaling factor for the  $Y_i$  we choose such that the average overall  $Y_i$  in the discrete regime is unity. As seen in fig 11(b&e) for the case of the average IS energy, determined via averaging over the density of states or via averaging over the simulation results, displays a perfect agreement with the direct average of the simulated energies. Finally,  $s_c(T) + \langle \ln Y_i \rangle$ , which is identical to  $\beta \langle E_{IS} \rangle + \ln \mathcal{Z}$  also does (basically) not depend on the choice of  $E_{cut}$ , see fig 11(c&f), implying a consistent calculation of the partition sum.

As outlined earlier, for system sizes  $N > 66$  and a given range of temperature, the bottom of the PEL is not identified, and thus a quantitative normalization of  $G(E_{IS})$  is not possible.

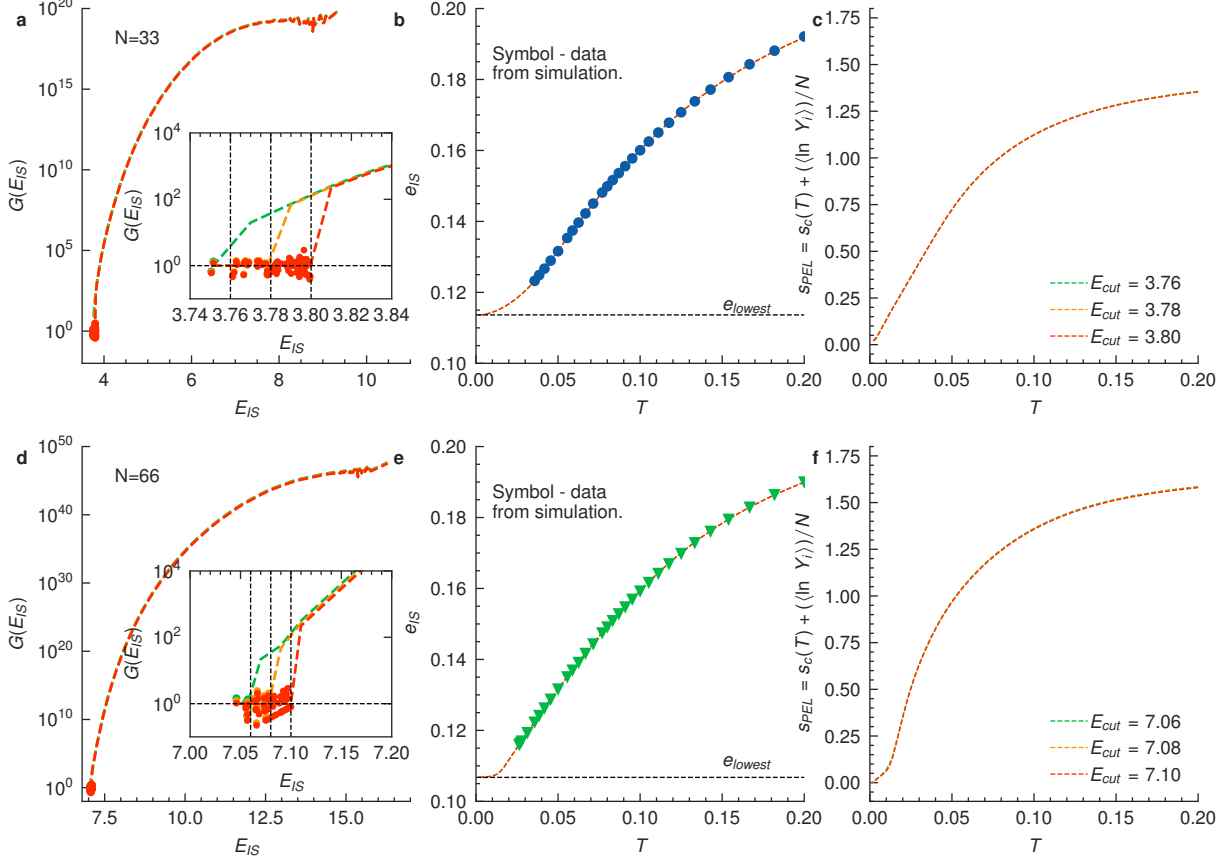

FIG. 11. **Thermodynamics of PEL.** **a & d** The  $G(E_{IS})$  for a range of choice for the cutoff ( $E_{cut}$ ). The calculation of the (**b & e**) potential energy of inherent structure and (**c & f**)  $s_c(T) + \langle \ln Y_i \rangle / N$ . The upper and lower panels represent the data for  $N=33$  and  $66$ , respectively.

Therefore,  $G(E_{IS})$  and thus  $\mathcal{Z}$  contains an unknown pre-factor. This results in an unknown shift of  $\ln \mathcal{Z}$ . Therefore, the total energy distribution can not be expressed in the absolute value, as done for  $N=33$  and  $66$  with unique bottom  $G(E_{IS,lowest}) = 1$  and  $\langle Y(T=0) \rangle = 0$ . As a consequence, the estimated  $G(E_{IS})$  would be off by a constant value. This would not affect the potential energy but only shift the entropy (see Fig. 11).

## X. FINITE-SIZE EFFECTS

### A. Energy

For temperatures above  $0.03$ , the average IS energy is basically  $N$ -independent. For  $N=33$  and  $66$ , the estimation can be extrapolated to  $T=0$ . Here one finds differences due to the

lower bottom, seen for  $N=66$ . Going above temperatures around  $T=0.15$ , minor finite-size effects are consistently seen. This is rationalized below.

## B. Basin properties in harmonic approximation

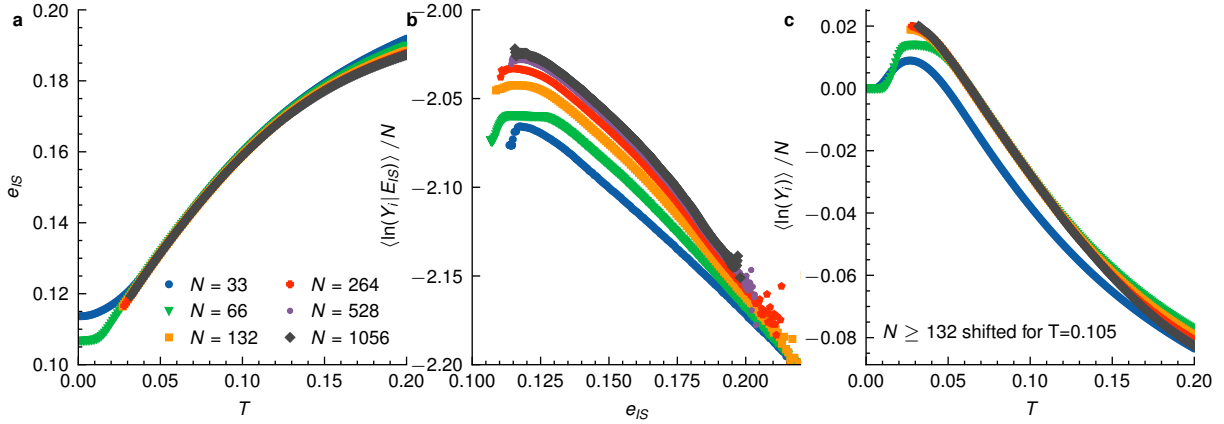

FIG. 12. **PEL and system size** (a) The mean potential energy for various system sizes is calculated from the partition sum. (b) The mean volume term vs. energy for various system sizes. (c) The temperature dependence of  $\ln Y$ , obtained from Boltzmann-averaging the energy-dependent terms in (b). For  $N=33$  and  $66$ , the Boltzmann-average can be extrapolated to zero temperature.

When analyzing the energy-dependence of the harmonic contributions, expressed by the average  $\langle \ln(Y|E_{IS}) \rangle$ , we find a qualitatively similar behavior, already known from other glass-formers [6]. The low-energy states possess larger  $Y$  and thus larger effective volumes. Surprisingly, there is a slightly non-monotonous behavior when approaching the bottom of the PEL. On a fully quantitative level, it turns out that larger systems display a larger effective volume, and only for system sizes of  $N=528$ , the macroscopic limit is reached. This may come as a surprise since the absolute number of states for  $N = 66$  is exponentially larger than expected from the  $N = 33$  system (see main text). Since the overall phase space per particle is identical, one might have expected the opposite trend (smaller effective basin for the larger system). This apparent discrepancy will be taken up again when discussing anharmonic effects. However, apart from a constant, the energy dependence is quite similar. As a consequence, when calculating the Boltzmann averaged value of  $\ln(Y)$ , the temperature

dependence is very similar. Here we have shifted the curves for  $N \geq 132$  to agree with the curve for  $N = 66$ . Since a scaling of the Y-values does not change the configurational entropy, this modification is fully appropriate. The residual variations (per particle) are of the order of 0.005 (for  $N \geq 66$ ) and 0.01 for  $N = 33$ . Indeed, such small violations from perfect finite-size scaling would be hardly visible in the configurational entropy (varying between 0 and 1, see main text). Thus, we may conclude that there are some finite-size effects in the effective volumes, estimated from the harmonic approximation. They are, however, too small to be relevant for the configurational entropy.

### C. Anharmonic effects

The per-particle anharmonic contribution to the average energy in a basin can be expressed as  $e_{anh}(T) = e_{liq.}(T) - e_{IS}(T) - (d/2)T$ , where  $e_{liq.}$  is the energy of the liquid,  $e_{IS}$  represents the energy of the inherent structure, and the last term is the harmonic contribution of the temperature. From  $e_{anh}(T)$ , we can write the anharmonic correction to the basin entropy

$$s_{anh}(T) = \int_0^T \frac{dT'}{T'} \frac{\partial e_{anh}(T')}{\partial T'}. \quad (21)$$

Since basins are increasingly harmonic at lower temperatures, one has  $e_{anh} = 0$  and  $s_{anh} = 0$  in the low-T limit. When the T-dependence of  $e_{anh}(T)$  is fitted by the low-temperature polynomial expansion,  $e_{anh}(T) = \sum_{i=2} \alpha_i T^i$ , Eq. 21 can be expressed as

$$s_{anh}(T) = \sum_{i=2} \frac{i}{i-1} \alpha_i T^{i-1}. \quad (22)$$

Fig. 13(a) shows the fit of order-8 for the  $e_{anh}$  for all system sizes. Starting with  $N = N_c = 66$ , there are only minor finite-size effects for  $T < 0.1$ , whereas the anharmonic effects are significantly stronger for  $N = 33$ . The strong decrease of  $e_{anh}$  with increasing temperature implies that in this temperature range, the effective volume is larger than expected from the harmonic approximation. This may explain, at least partly, why for  $N = 33$ , both the absolute number of states and the effective volume per basin, estimated via the harmonic approximation, are smaller than for  $N = 66$ , whereas the opposite would have been expected when considering the same total phase space volume per particle. The

corresponding anharmonic contributions to the entropy ( $s_{anh}$ ) are shown in Fig. 13(b).

In general, the anharmonic effects modify the  $Y_i$ , obtained within harmonic approximation. Thus, in general, one may write (when concentrating on the average  $Y(E)$ ) that  $Y_{tot}(E) = Y_{harm}(E) \cdot Y_{anh}(E, T)$ . For purely harmonic systems, one would have  $Y_{anh}(E, T) = 1$ . The additional temperature dependence for  $Y_{anh}(E, T)$  implies that in contrast to the harmonic approximation, the temperature dependence cannot be simply scaled out but may appear in a more complicated way.

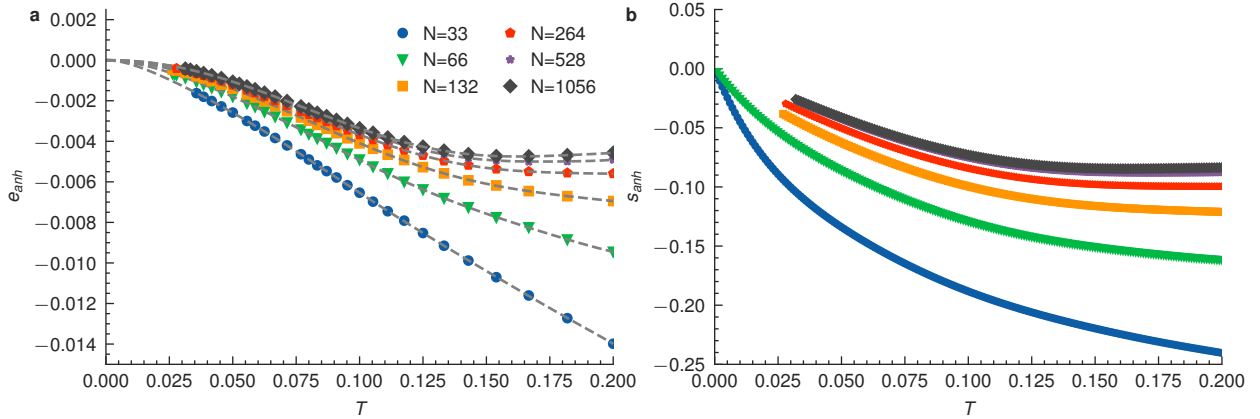

FIG. 13. **Anharmonic corrections** (a) The anharmonic contribution in the potential energy and (b) entropy across the system sizes.

The anharmonic effects, discussed above, yield information about the individual basins. They would modify  $S_{vib}$ . However, if the temperature dependence of  $Y_{anh}(E, T)$  appears in a separate factor (as for the harmonic approximation), the anharmonic corrections would be irrelevant for the present approach to estimate the configurational entropy. The reason is the insensitivity of the configuration entropy to the scaling  $Y_i \rightarrow \lambda Y_i$  (see above). If, however, they would not simply scale out, the reweighting procedure, to obtain the volume-weighted density of states  $G(E)$  would not work. As shown in (SI II) no significant deviations are present. Thus, we may conclude that anharmonic effects are irrelevant to the estimation of the configurational entropy via the Shannon formula. As is well known, in the limit of high temperatures beyond the onset-temperature anharmonic effects start to matter, and a unique construction of a volume-weighted IS density is no longer possible.

### D. Configurational entropy

So far we have shown that for  $N \geq 66$  all ingredients, entering the configuration entropy, display very minor finite effects, namely  $\langle \ln Y \rangle$ ,  $\langle e_{IS} \rangle$ , and the partition sum. The statement about the partition sum is concluded from the validity of the superposition hypothesis as discussed in the main part (except for one overall constant). As a consistency check, we show the configurational entropy (already seen in the main text) in fig 14. Furthermore, we present its derivative with respect to temperature which is more sensitive to possible finite-size effects. Remarkably, also the derivative is identical for all system sizes  $N \geq 66$ . Here no scaling was required to match  $N = 66$  with  $N \geq 66$ . Thus, one can indeed conclude that for  $T > T_g/2$  the thermodynamics of the  $N = 66$  system, as expressed by the configurational entropy, already reflects the macroscopic limit.

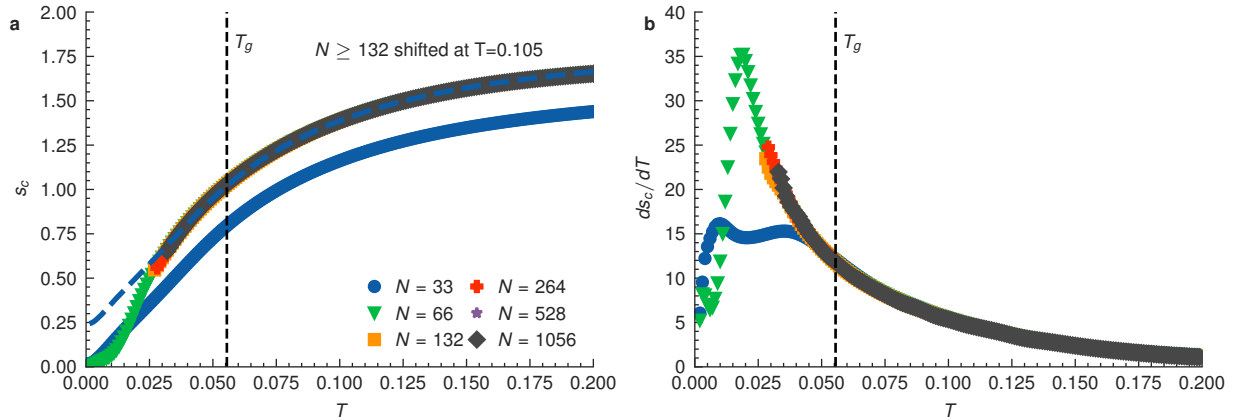

FIG. 14. **Configurational entropy and system size** (a) The configurational entropy for all  $N$ , is studied in this work. The curves for  $N > 66$  have been shifted so that they agree with the curve for  $N = 66$  at  $T = 0.105$ . (b) The temperature derivative of the configurational entropy.

### E. Minimalist model to rationalize the corrections to the superposition hypothesis for the absolute number of IS

As discussed in the main text, the absolute number of IS for the  $N = 66$  system is larger by a factor of nearly  $10^7$  as expected from the superposition hypothesis. The relative increase is independent of energy (except for the low-energy end). This observation can be rationalized for a minimalist model system.

We consider a system of  $N_A$  particles of type A and  $N_B$  particles of type B and a total number of  $N$ . The total permutations of  $N$  particles, while considering  $N_A$  and  $N_B$  identical, can be expressed as

$$W = \frac{N!}{N_A!N_B!} \quad (23)$$

If all states have the same energy, the configurational entropy can be expressed via the number of micro-states  $S_c = k \ln W$ , where  $W$  is the number of possible configurations for a system. Thus, the entropy can be expressed as

$$S_c = \ln N! - \ln N_A! - \ln N_B! \quad (24)$$

With the Stirling approximation, this can be rewritten as

$$\begin{aligned} S_c &= N \ln N - N + \frac{1}{2} \ln N + N_A \ln N_A - N_A + \frac{1}{2} \ln N_A + N_B \ln N_B - N_B + \frac{1}{2} \ln N_B \\ &= -N_A \ln \frac{N_A}{N} - N_B \ln \frac{N_B}{N} + \frac{1}{2} \ln \frac{N}{N_A N_B}. \end{aligned} \quad (25)$$

On this basis, the per-particle configurational entropy can be expressed as

$$s_c = -p_A \ln p_A - p_B \ln p_B - \frac{1}{2N} \ln N - \frac{1}{2N} \ln p_A p_B, \quad (26)$$

where  $p_A$  and  $p_B$  are the fractions of the A and B type subsystems, respectively. This straightforward observation suggests the dominant finite-size effects in the entropy are proportional to  $(\ln N)/N$  and have a negative sign.

Thus, there is a generic finite-size scaling that may be relevant up to quite large values of  $N$ . This may explain why there is this significant temperature-independent positive shift in entropy when comparing  $N = 33$  and  $N = 66$ . For, e.g.,  $T=0.1$ , this is definitely unrelated to the deviations close to the bottom of the PEL. Strictly speaking, compared to  $N=33$ ,  $N=66$  would have roughly  $\exp(66\Delta s_c)$  states. At the high temperature, the difference is roughly constant with value  $\Delta s_c (= s_{c,N=66} - s_{c,N=33}) = 0.225$ , corresponds to  $10^{6.5}$  excess-states for  $N=66$ . Furthermore, this observation suggests that this will hold for even larger system sizes and may be rationalized by simple statistical considerations as done for this minimal model. Most importantly, the ability to superpose the configurational entropy for  $N = 33$  and  $N = 66$  for  $T > T_g$  (after shifting) shows that, first, the deviations of the

PEL at very low energies are irrelevant for the thermodynamics at  $T > T_g$  and, second, the remaining IS density is nearly identical for both system sizes apart from an overall scaling factor.

## XI. OBSERVATIONS IN EXPERIMENTAL SYSTEMS FOR THE FSC

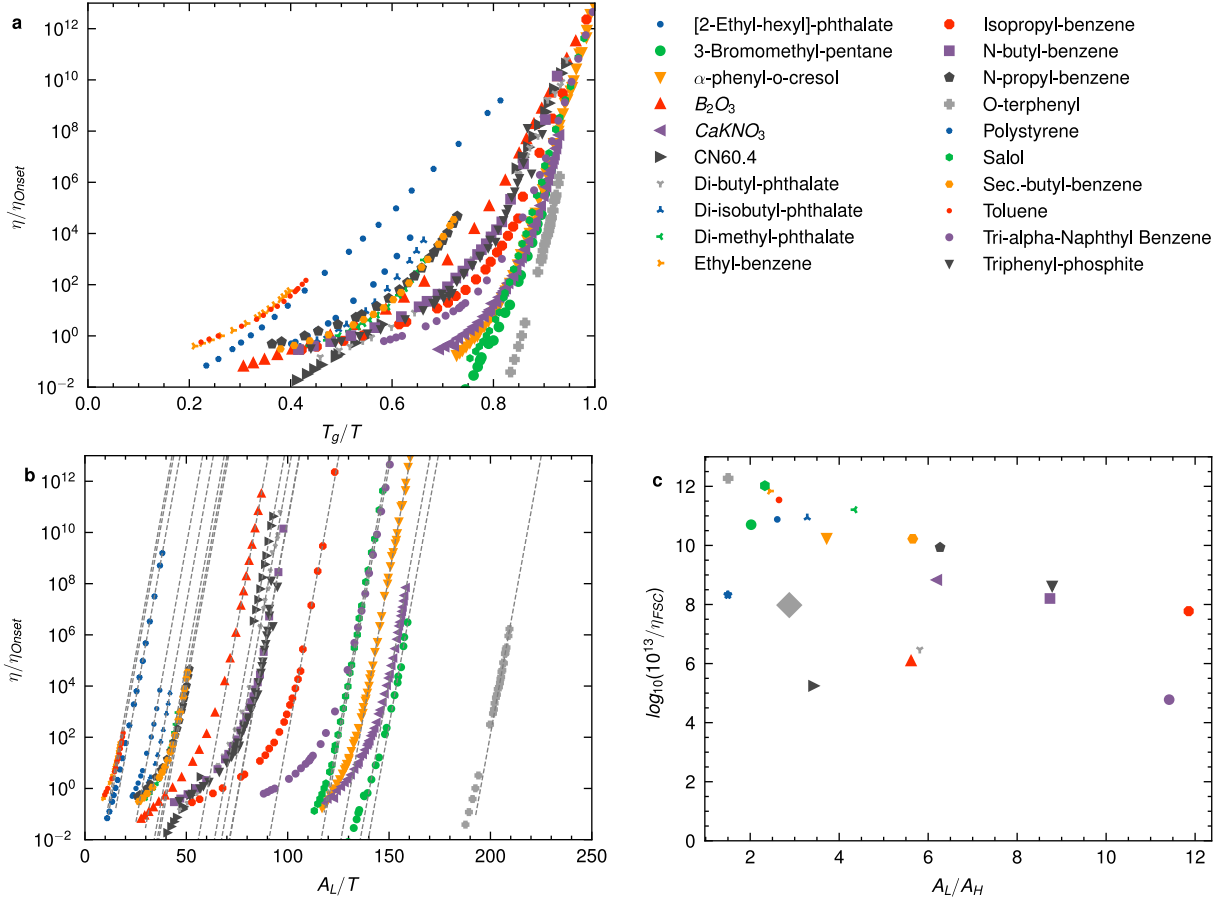

FIG. 15. **FSC with experimental system** The fragile to strong crossover is a general glassy observation for different experimental systems. (a) Angell's representation of the studied system, (b) The quantification of the Strong behavior in the supercooled regime of the system. (c) The complication of the overall range of Arrhenius-like relaxation (compared with  $T_g$ ) against the scaled activation energy. The large gray symbol corresponds to the structural relaxation time for  $N=1056$ , showing the "strong" relaxation till  $T_g$ , defined as  $\tau_\alpha(T_g) = 10^{12}$ .

In the context of the fragile-to-strong crossover, we have compiled a range of experimental *non-network forming* supercooled systems which clearly show an Arrhenius-behavior at low

and high temperatures, see Fig. 15. This corroborates the study by Mallamace et al. [7]. A better comparison is possible when plotting the scaled viscosity vs. the ratio of the low-temperature activation energy ( $A_L$ ) and the high-temperature activation energy ( $A_H$ ). Except for a few cases, one observes a clear correlation of  $A_L/A_H$  with the viscosity at the fragile-to-strong crossover. The model system, studied in this work, displays a value of  $A_L/A_H \approx 2.88$  (for the structural relaxation) and is thus in the range of experimentally observed values. This highlights the relevance of the current findings also in the context of the interpretation of experimental results.

- 
- [1] A. Ninarello, L. Berthier, and D. Coslovich, *Physical Review X* **7**, 021039 (2017).
  - [2] J. D. Ferry, *Viscoelastic properties of polymers* (John Wiley & Sons, 1980).
  - [3] Y. S. Elmatad, D. Chandler, and J. P. Garrahan, *The Journal of Physical Chemistry B* **114**, 17113 (2010).
  - [4] L. Berthier and M. D. Ediger, *The Journal of Chemical Physics* **153**, 044501 (2020).
  - [5] L. Berthier and G. Biroli, *Reviews of modern physics* **83**, 587 (2011).
  - [6] S. Büchner and A. Heuer, *Physical Review E* **60**, 6507 (1999).
  - [7] F. Mallamace, C. Branca, C. Corsaro, N. Leone, J. Spooren, S.-H. Chen, and H. E. Stanley, *Proceedings of the National Academy of Sciences* **107**, 22457 (2010).
